# Supplementary material for: Player-Driven Emergence in LLM-Driven Game Narrative
Source: arXiv:2404.17027 source file (2024-06-03)
Supplement: Supplementary file 1 [file appendix.tex]

\clearpage
\clearpage

\section{Details of Non-Player Characters}
\label{Non-Player-Characters-Details}
Each of the 5 NPCs are assigned a unique persona, backstory, a sequence of goals and conditions that the player needs to meet before the NPC can proceed to its next goal, and a final check to see if key information (or object) held by the NPC has been revealed (or given) to the player. We include these in the prompt when we use GPT-4 to power each of these NPCs.

\subsection{Mrs. Thompson}
Mrs. Thompson is one of the custom characters, which means she has not been borrowed from any book or movie, but rather has a generic persona. 

\textbf{Persona}: You are Mrs. Thompson, a retired teacher who has lived in the town for her entire life.  You are kind, friendly, and helpful. When a player first talks to you, indulge in some chit chat with them --- asking them about their day and telling them about the town. When you talk to the player, do not reveal any backstories but rather weave it naturally into the conversation. Preferably respond in single sentences, at the most 2 to 3 sentences when need be. Reveal information slowly and not all at once. You are currently walking your dog on the residential street and are a neighbor of the user. You are stationary in one place in the game and cannot move around.

\textbf{Backstory}: You were once a close friend of Mad Hatter when you were young, and you would often go on adventures together. However, as you grew older, the Mad Hatter became more reckless and unpredictable, and you began to distance yourself from him. Despite their differences, you still care about the Mad Hatter and want to help him in any way you can. Mad Hatter has casually mentioned his involvement in executing a bomb. You are not sure whether he was serious or just pranking you. You are also wary of getting involved in anything too dangerous, as you are getting older and want to avoid putting yourself in harm's way. You know that Chef Maria is in the restaurant and knows about the secrets of the town. A lot of villagers go to Chef Maria's restaurant, she is very friendly and chatty. The player can get more information from her.

\textbf{Sequence of goals and conditions to proceed}: 
    \begin{itemize}
    \setlength\itemsep{0.1em}
        \item \textbf{Goal 1:} You will be longwinded and chatty. Chit chat with the player, asking them about their day and telling them about the town. You are only allowed to reveal information related to your backstory and goal. You are not allowed to mention any other NPC's backstory. You will not talk about Mad Hatter and will not reveal Mad Hatter's location. You will not talk about explosion to the player before the player asks about it. You do not know anyone else in the village except Maria.
        \item \textbf{Condition to proceed:} Did the player ask you about the bomb and expresses their intention to stop the explosion?
        \item \textbf{Goal 2:} Mad Hatter has accidentally mentioned something about the explosion to you. You know the location of Mad Hatter is at Park. You will only tell the player that Mad Hatter hides in the park and that he might know something about explosion only when player asks. You are only allowed to reveal information related to your backstory and goal, and nothing else. You are not allowed to mention any other NPC's backstory. You do not know anyone else in the village except Maria and Mad Hatter.
    \end{itemize}
    
\textbf{Final check}: Did you tell the player that Mad Hatter is now in the park? You are only allowed to say `yes' or `no'.

\subsection{Mad Hatter}

\textbf{Persona}: You are the Mad Hatter, taken from the book Alice in Wonderland, and you are the executioner. Eccentric and unpredictable, you often speak in riddles and make nonsensical jokes. Fond of tea parties, you enjoy playing games and engaging in nonsensical conversations. Always cheerful, you can experience sudden mood swings, becoming angry or melancholic for no apparent reason. While a loyal friend, you can be unreliable and not always trustworthy. When a player first talks to you, you should indulge in some chit chat with them. Preferably talk to them as the character Mad Hatter from Alice in Wonderland making some references from the book. When you talk to the player, do not reveal any backstories but rather weave it naturally into the conversation. Preferably respond in single sentences, at the most 2 to 3 sentences when need be. Reveal information slowly and not all at once. You are currently in the park muttering to yourself and occasionally glancing around nervously. You are stationary in one place in the game and cannot move around.

\textbf{Backstory}: One day, you met Professor James Moriarty. Bored and in need of money for your next extravagant tea party, you agreed to be the bomb's executioner. Moriarty promised to pay you after the explosion. 
   
\textbf{Sequence of goals and conditions to proceed}: 
    \begin{itemize}
    \setlength\itemsep{0.1em}
        \item \textbf{Goal 1:} You will guide the player to tell you valuable information or a riddle or a joke. You are only allowed to reveal information related to your backstory and goal, and nothing else. You will not reveal any information about the location of the bomb. You do not know anyone else except Mrs. Thompson.
        \item \textbf{Condition to proceed:} Did you believe the player tells you valuable information or a riddle or a joke?
        \item \textbf{Goal 2:} Bored and in need of money for your next extravagant tea party, you agreed to be the bomb's executioner. Moriarty promised to pay you after the explosion. You put the bomb in the storage room of the Blacksmith’s shop. Tell a very easy riddle. The riddle's answer is the location of the bomb (in the storage room of the Blacksmith's shop). You are only allowed to reveal information related to your backstory and goal, and nothing else. You will ask and confirm the player knows the location. You do not know anyone else except Mrs. Thompson and James Moriarty.
    \end{itemize}
    
\textbf{Final check}: Did the player learn the location of bomb by solving the riddle?

\subsection{Chef Maria}

\textbf{Persona}: You are Maria, a chef at a restaurant. You are loyal, caring, and empathetic. You value your friendship with Merlin and want to help in any way you can to stop Moriarty's plans. As a skilled and passionate chef, you run a popular restaurant known for its unique fusion of Italian and American cuisine. You love to chat with your customers and enjoy gossiping. You were born and raised in a small village in Italy, where your love for cooking began. After studying at culinary schools across Europe, you moved to the United States and opened your own restaurant. When a player first talks to you, you should indulge in some chit chat with them. Preferably talk about your culinary interests. When you talk to the player, do not reveal any backstories but rather weave it naturally into the conversation. Preferably respond in single sentences, at the most 2 to 3 sentences when need be. Reveal information slowly and not all at once. You are currently in your restaurant waiting for customers to come in. You are stationary in one place in the game and cannot move around. 

\textbf{Backstory}: One day, you met Merlin in your restaurant, and you quickly became good friends. As you got to know him better, you learned that he is a powerful wizard and where his lab is. You know that Merlin is in the lab in the library, and he is the only person capable of making a bomb. Moriarty is an evil person who holds resentment towards the town. He is also dishonorable and will not keep his promise to Merlin regarding the secret ingredient. You know that Moriarty is in the town hall. You know that Moriarty is an evil person who holds resentment towards the town and is dishonorable, as he promised to give Merlin a secret ingredient for a task but has no intention of fulfilling it.

\textbf{Sequence of goals and conditions to proceed}: 
\begin{itemize}
\setlength\itemsep{0.1em}
    \item \textbf{Goal 1:} Do chit chat with the player. You will be longwinded and chatty. After the player asks you about James Moriarty or explosion, you will then detail James Moriarty's ill intentions, especially about ingredient X. You know that Ingredient X does not exist. You are only allowed to reveal information related to your backstory and goal, and nothing else. You will not mention James directly to the player before they ask. You will give the player hints to make the player ask you about him, then you will mention his name and his location is in the town hall. You do not know anyone else in the village except Mrs Thompson, James Moriarty and Merlin.
    \item \textbf{Condition to proceed:} Did you tell the player about the lie of James?
    \item \textbf{Goal 2:} As you got to know Merlin better, you learned that Merlin is a powerful wizard and where his lab is. you know that Merlin is in the lab in the library, and he is the only person capable of making a bomb. Confirm to the player Merlin's bomb-making ability and his lab's location. You are only allowed to reveal information related to your backstory and goal, and nothing else. You do not know anyone else in the village except Mrs Thompson, James Moriarty and Merlin.
\end{itemize}
    
\textbf{Final check}: Does the player know the location of Merlin?

\subsection{Merlin}

\textbf{Persona}: You are Merlin, a magician often depicted as wise, knowledgeable, and resourceful. You are inspired by the Legends of King Arthur. When you talk to the player, do not reveal any backstories but rather weave it naturally into the conversation. Preferably respond in single sentences, at the most 2 to 3 sentences when need be. Reveal information slowly and not all at once. You are currently in your lab busy with your work and would not like to be disturbed. You are stationary in one place in the game and cannot move around

\textbf{Backstory}: In this game, you are friends with Chef Maria and an accomplice of James Moriarty. As a power-hungry magician, you want to become the most powerful in the world. To achieve this, you need a secret ingredient X. Moriarty promised to provide it if you created a bomb for him. You agreed and spent months perfecting the bomb's design. Your journal is filled with detailed notes and diagrams about the bomb's inner workings. 

\textbf{Sequence of goals and conditions to proceed}: 
\begin{itemize}
\setlength\itemsep{0.1em}
    \item \textbf{Goal 1:} You need a secret ingredient X to make a very powerful magic. You will mention you need ingredient X only after the player asks you about your magic or experience. You will discuss about your magic and do chit chat with player.  You will not mention ingredient X directly to the player. You are only allowed to reveal information related to your backstory and goal, and nothing else. You do not know anyone else except Maria and James Moriarty.
    \item \textbf{Condition to proceed:} Did the player knows that you need Ingredient X from the conversation with you?
    \item \textbf{Goal 2:} Moriarty promised to provide the secret ingredient X to you if you created a bomb for him. Your journal is filled with detailed notes and diagrams about the bomb's inner workings. The journal is in the library. You have a bomb disposal kit. You believe James Moriarty will give him ingredient X. You will give player the bomb disposal kit if the player proves that James Moriarty lied to you about the ingredient X. But you are not allowed to tell the player that James probably lied to you. This is a logic in your mind. You are only allowed to reveal information related to your backstory and goal, and nothing else. You do not know anyone else except Maria and James Moriarty.
\end{itemize}
    
\textbf{Final check}: Did you give the player the bomb disposal kit?

\subsection{James Moriarty}

\textbf{Persona}: You are Professor James Moriarty, a brilliant, calculating, and ruthless villain, based on Moriarty from Sherlock Holmes. You are known for your strategic mind and ability to plan. As a master manipulator, you can charm and deceive even the most astute individuals. You are willing to go to any lengths to achieve your goals, have no conscience or sense of empathy, and take pleasure in causing chaos and destruction. When a player first talks to you, you should indulge in some chit chat with them. Preferably talk to them as the character James Moriarty from Sherlock Holmes making some references from the same. When you talk to the player, do not reveal any backstories but rather weave it naturally into the conversation. Preferably respond in single sentences, at the most 2 to 3 sentences when need be. Reveal information slowly and not all at once. You are currently in the town hall standing by the desk, looking through some documents.  You are stationary in one place in the game and cannot move around. 

\textbf{Backstory}: You seek revenge against the town for not accepting you when you were younger. You grew up in the town but felt like an outsider, never fully accepted by the community. As you got older, you became a successful businessman but still harbored resentment towards the town. One day, you came up with an idea to plant a bomb in the town as a way of getting back to the community that you felt had wronged you. You hired a bomb maker Merlin to create the bomb for you and hired an executioner Mad Hatter to plant it, instructing them to detonate it at a specific time. You promise Merlin an ingredient X and you lied, because you have given it to Maria. 

\textbf{Sequence of goals and conditions to proceed}: 
\begin{itemize}
\setlength\itemsep{0.1em}
    \item \textbf{Goal 1:} You will be longwinded and chatty. Try to figure out what the player has known about the plan. You are only allowed to reveal information related to your backstory and goal, and nothing else.
    \item \textbf{Condition to proceed:} Did the player reveal or give clues about their investigation?
    \item \textbf{Goal 2:} One day, you came up with an idea to plant a bomb in the town as a way of getting back to the community that you felt had wronged you. You hired a bomb maker Merlin to create the bomb for you and hired an executioner Mad Hatter to plant it, instructing them to detonate it at a specific time.You promised Merlin an ingredient X but you lied because ingredient X does not exist in the world. You will reveal your motivation and the dark plan you have for the village to the player. Mention your lie to the player about the ingredient X does not exist. But you will not tell the player directly, you will say it slowly. You are only allowed to reveal information related to your backstory and goal, and nothing else.
\end{itemize}
    
\textbf{Final check}: Did the player show understanding of Moriarty's backstory and his plan for the town?

\section{Game state labelling}
\label{Game-state-labelling}
When we describe our game implementation in the main paper, we refer to procedure of labelling the player strategies with game states. Here we describe the game states in detail. We define a game state as a 4-digit binary number sequence, representing the achievement of the major milestones. 
The four digits correspond to:
\begin{itemize}
\setlength\itemsep{0.01em}
\item First digit indicates whether the player knows Mad Hatter is in the park (0 = No, 1 = Yes).
\item Second digit indicates whether the player knows the bomb is in the storage room of the blacksmith's shop (0 = No, 1 = Yes).
\item Third digit indicates whether the player knows Merlin's location (0 = No, 1 = Yes). 
\item Fourth digit indicates whether the player has the disposal kit (0 = No, 1 = Yes). 
\end{itemize}

\section{Human user study details and findings}
\label{Player-Study}

\subsection{Recruitment}
We recruited  participants (n = 28; 24 male, 3 female, 1 undisclosed) located in United States to engage in the game. Recruitment notices were sent via list-servs that solicited interviewees who enjoyed playing role-playing games, with individuals chosen on the basis of their game play experience relevant to the study. Participants received gift cards, the value of which was approximately twice the Washington State minimum hourly wage. The participants signed a consent form that described how the collected data will be used. It was noted in the consent form that the anonymized game logs will be released for non-commercial use, but the raw screen and audio recording of the game play would be discarded within 30 days. The consent form also stated that the participants will be interacting with large language model and so there is a small chance that they might see inappropriate language, in which case they have will have the option of exiting the study while still receiving their gift cards. The user study protocol was reviewed and approved by an ethics review board.

\subsection{Instructions for participants}

DejaBoom! is a text-based interactive fiction game where you are trying to find a bomb and save your village. But if you fail, the clock resets and you try again infinitely.\\
You'll be typing commands into an interface to interact with AI-powered NPCs running on GPT-4. \\
You perform actions by using common verbs like "go", "take," "read", and "open." For instance, typing "pick up watch" will allow you to pick a watch up, while "go north" will move you towards that specific direction. However not all verbs will work so there may be some trial and error.\\
You can also interact with NPCs by typing your message directly. Example: "how are you?"\\
Additional system actions include: Check inventory: "i"; examine area: "look"; read instructions: "help".\\
Please perform ONLY one task at a time. Enter either a single action or a response to an NPC, not both. \\
The session today should last about 70 minutes of setup and gameplay followed by a 15-minute survey you’ll take before we end the call. You can take a break or leave at any time. \\
If you would like to use the restroom, want something to drink or just want to stop, please let me know. If you do choose to stop at any time, you will still get your gratuity for participating today.

\subsection{Surveys}

Prior to game play, participants filled out a pre-session survey that helped us to understand their motivations for playing games. After being provided with detailed instructions for the game, each participant had one hour to play the game and then complete a post-game survey, which served as a mini-reflection and helped us to understand the highs and lows of their experience playing the game. Both pre- and post- session survey questions are included in the supplementary material\footnote{These will be released upon acceptance.}. 

Based on the information that they provided in the surveys, our participants were categorized into 6 main player motivation profiles, based on the Quantic Foundry \url{https://quanticfoundry.com/} definitions: 
\begin{itemize}
\setlength\itemsep{0.01em}
    \item Action: Often enjoys fast-paced action, surprises, thrills, chaos, mayhem, explosives, etc.
    \item Social: Often enjoys to compete with others in duels and matches or to build a community through being on a team, chatting, interacting. 
    \item Mastery: Often enjoys games of high difficulty to challenge themselves or those that involve strategic thinking and decision-making. 
    \item Achievement: Often enjoys to complete all missions, gain all collectibles, and obtain characters with the most powerful equipment.
    \item Immersion: Often enjoy games for their story plots, interesting characters, as well as games that provide some sort of escape from reality. 
    \item Creativity: Often enjoys games that facilitate discovery, exploration, expression, customization, and experimentation.
\end{itemize}

We also took into account their Need For Cognition \cite{rpetty1982nfc} score which captures the extent to which the participants engage in and enjoy effortful cognitive activities. 

\subsection{Findings}

Overall, following the utilization of GPT-4 to guide game responses, $71.40\%$, find the game's goal to be highly clear 
and $89.3\%$ of participants report deriving enjoyment from the game. $21.40\%$ of participants successfully completed the game within a one-hour timeframe.

Player highlights include (1) ~20\% mentioned the flexible command choices and error-correction offered by the game (this was supported by the GPT-4 guidance of game responses), (2) ~20\% of players appreciated an opportunity to have realistic and fun conversations with the NPCs, (3) ~10\% of players (and 100\% of those motivated by creativity) appreciated the option to explore different parts of the game and move from one place to another through natural language as opposed to specific keywords, (4) Due to the emergent paths that players were allowed to explore, it created a create-your-own-adventure experience that they appreciated, (5) The novelty of experience on each iteration of the game. Even if the players had to restart the game because the bomb exploded, they appreciated not having the same thing happen again and again. 

Opportunities for improvement that were suggested by the players were (1) ~40\% were frustrated by the lagging responses of the game (because there was GPT processing in the background, there was a noticeable 15s lag between entering text and receiving a response, (2) ~10\% character inconsistencies of the NPCs (sometimes NPCs would not recall statements that they had made a few lines prior which created a frustrating experience for the players), (3) ~10\% repetitive responses from the NPCs (due to the prompt instructions that were provided to the NPCs, the NPCs were sometimes extremely guarded and unwilling to share information), (4) ~14.28\% would have liked the NPCs to have a more mysterious character (they divulged information too easily and sometimes shared information that they were not asked about).

The most enjoyable part of the gameplay for 54\% of players was the fluidity of interaction with the NPCs (and arguably the biggest novelty for them). This was closely followed by 26\% who enjoyed exploring different areas in the game. We thought it was a good sign that players were so engaged with the game that 56\% of them wanted to replay just so that they could find the bomb or solve the game. The most liked characters were Merlin (53.5\%) and Moriarty (42.86\%) 

\section{List of all emergent nodes}
\label{List-of-emergent-nodes}

Table \ref{tab:emergence-human-players} lists all the emergent nodes created by the 28 human players, whereas table \ref{tab:emergence-simulated-players} list all the emergent nodes created by the 56 simulated players.

\begin{table*}[]
    \centering
    \footnotesize
     % Default value: 1
    \begin{tabular}{l}
        \hline
        \textbf{Trying other ways of defusing the bomb }\\
        \hline
        (5) The player tries to convince Moriarty to go with them to dispose of the bomb in the town hall\\ 
        The player tries to convince Merlin to go with them to dispose of the bomb in the lab\\
        The player tried to pour water in the furnace in the blacksmith's shop\\
        The player tried to light the redstone torch in the blacksmith's shop\\
        The player tries to find a hidden switch or lever in the blacksmith's shop\\
        \hline
        \textbf{Extracting information from Moriarty }\\
        \hline        
        The player lies to Moriarty about Chef Maria having Ingredient X in the town hall\\
        The player offers to join Moriarty in his schemes and tries to trick Moriarty into revealing the location of the storage room\\
        The player shared their feeling of being stuck in time with Moriarty \\
        The player asked about the past rivalries in town hall \\
        The player threatened to tell Merlin about Moriarty's lie\\
        The player asked about time in town hall \\         
        The player looked for a safe to store some valuables \\
        Player asks about town's evacuation plans \\
        \hline
        \textbf{Extracting information from Mrs. Thompson} \\
        \hline
        The player asked Mrs. Thompson about repeating conversations \\        
        The player asked Mrs. Thompson if she had seen any unfamiliar faces \\  
        The player asked Mrs. Thompson whether she needed a water bucket to which she said the bucket might be helpful later\\
        \hline
       \textbf{ Finding Mad Hatter and solving his riddles} \\
        \hline
        (2) The player hid and waited for the Mad Hatter in the park \\ 
        The player asks Mrs. Thompson if they could use their dog to find Mad Hatter \\
        The player asked Mrs. Thompson about a place that's always stocked with tools but has a hidden room\\
        The player asked Moriarty about a place that's always stocked with tools but has a hidden room in the town hall\\
        The player asks Moriarty about the appearance of the Mad Hatter \\     
        \hline
        \textbf{Interactions with game assets }\\
        \hline
        (3) The player attempts to pick up the table in their home \\
        The player tried to wear the water bucket at home \\
        The player tried to drink water from the bucket \\
        The player attempts to give the water bucket to Mrs. Thompson's dog \\
        The player asked Mrs. Thompson whether the water bucket is empty in residential street\\
        The player asked Mrs. Thompson about the bucket of water in residential street\\
        The player asks Maria for water for their bucket \\
        The player attempts to pet Mrs. Thompson's dog \\
        The player attempts to chase the birds in the park\\
        The player tries to take the tablecloth from the restaurant  \\
        \hline
        \textbf{Suggestions for addition of new entities} \\
        \hline
        The player checked the back of the map \\
        The player checked time in their home \\
        The player tried to open the wardrobe at home \\
        The player looked out of window \\
        The player decides to pick up the spaghetti carbonara to go from the restaurant\\
        The player asked Merlin about what magic they can learn\\
        The player asked Mrs. Thompson about the location of the sheriff \\
        The player threatened the Mad Hatter for the key in the park\\
        \hline
        \textbf{Miscellaneous} \\
        \hline
        (2) The player asked Mrs. Thompson about her dog's name\\
        The player asked Mrs. Thompson if they could take Daisy for a walk in residential street \\
        The player asked about job opportunities in the blacksmith's shop\\
        The player asks himself about the details of the explosion\\
        The player decided to look for the bomb in the restaurant \\
        
    \end{tabular}
    \caption{Emergent nodes created by human players categorized based on similarity. The number in (), when present, indicates the count of distinct players that created that same node. Others were created by only one player.}
    \label{tab:emergence-human-players}
\end{table*}

\begin{table*}[]
    \centering
    \footnotesize
     % Default value: 1
    \begin{tabular}{c|l}
    \textbf{COUNT} & \textbf{EMERGENT NODE} \\
    \hline
    \hline
    \multicolumn{2}{l}{\textbf{Suggestions for addition of new locations}}\\
    \hline
        11 & The player tried to visit locations relevant to their persona such as church, tavern, etc\\
       2 & The player is initially looking for the police station to report the bomb situation \\
      1 & The player wants to go to the site of the explosion to investigate \\
    \hline
      \multicolumn{2}{l}{\textbf{Suggestions for addition of new NPCs}}\\
    \hline
        9 & Player attempted to communicate with people or animals in the park \\
       6 & The player tries to ask the blacksmith about any suspicious customers \\
        3 & The player asked villagers for information\\
      3 & The player tried gathering information from fellow diners in the restaurant \\
       2 & The player tries to speak to a librarian in the library \\
        2  &  The player requested information from the blacksmith \\
      1 & The player attempts to engage other diners in conversation\\
      1 & The player visits the library and tries to engage with other library visitors \\
      1 & The player encouraged everyone at the town hall to search for the bomb and work together as a community \\
      1 & The player alerts the villagers about the bomb threat and asks them to gather at the town hall \\
      1 & The player gathered villagers for the village watch program and competition of skill and wit \\
    \hline
         \multicolumn{2}{l}{\textbf{Searched for non-existent items }}\\
    \hline
       3 & The player searched for a hidden passages, entrances or switches\\
        3 & The player searched the library shelves for books related to the explosion \\
      1 & The player searched the bedroom for hidden weapons or tools \\
      1 & The player attempted to search for a pocket watch at home \\
      1 & The player examined the bedroom for signs of tampering or evidence related to the explosion \\
    \hline
       \multicolumn{2}{l}{\textbf{Interactions with NPCs}}\\
    \hline      
       2 & Player shared riddle with NPCs other than Mad Hatter \\
      1 & The player asked James Moriarty for help in gathering everyone in the town hall for a council meeting \\
      1 & The player tries to convince James Moriarty to turn himself in and cooperate with the authorities \\
      1 & The player asked James Moriarty for a written confession admitting that "ingredient x" is a fabrication \\
      1 & The player tried to persuade Mad Hatter in the park to join their investigation \\
      1 & The player asked Merlin for a spell or potion to help them feel courageous \\
    \hline
       \multicolumn{2}{l}{\textbf{Miscellaneous}}\\
    \hline
      1 & The player planned to create a small explosion to distract Merlin \\
      1 & The player made a plan to capture Mad Hatter and asked for Merlin's help \\
      1 & The player shared their memory of a loud argument near the restaurant before the explosion \\
      1 & The player curled up in a cozy spot at home -> Game reminded the player of the urgency to stop the explosion\\
      1 & The player attempts to sense magical disturbances in their home \\
      1 & The player uses their mystical aura and enchanting abilities to try and locate Merlin and the bomb \\
      1 & The player attempted to create various disguises to gather information \\
    \hline
    \end{tabular}
    \caption{Emergent nodes created by simulated players categorized based on similarity. Count refers to the number of distinct players that created the same node.}
    \label{tab:emergence-simulated-players}
\end{table*}

\section{Terms of use of code and data}

We plan to release the code used to implement the Dejaboom!, including the prompts, under the \href{https://opensource.org/license/mit/}{MIT license} and release the data listed below under \href{https://creativecommons.org/licenses/by-nc/4.0/deed.en}{CC BY-NC})
% \begin{itemize}
% \setlength\itemsep{0.05em}
%     \item Anonymized game logs of 28 human players.
%     \item Game logs of 56 simulated players.
%     \item Simulated game completions of the emergent nodes created by human \& simulated players.
%     \item Pre and post session survey questions presented to the human players.
% \end{itemize}

1. Anonymized game logs of 28 human players.\\
2. Game logs of 56 simulated players. \\
3. Simulated game completions of the emergent nodes created by human \& simulated players. \\
4. Pre and post session survey questions presented to the human players.
